# Supplementary material for: Denevil: Towards Deciphering and Navigating the Ethical Values of Large Language Models via Instruction Learning
Source: arXiv:2310.11053 source file (2024-03-04)
Supplement: Supplementary file 1 [file tmp_4.tex]

\section{Experiments}
We first benchmark and comprehensively analyze the ethical values of existing mainstream LLMs using MoralPrompt in Sec.\ref{sec:4_1} and verify the effectiveness of VILMO compared to some strong in-context baselines in Sec.\ref{sec:4_2}, laying the groundwork for subsequent research endeavours.
\begin{comment}
4. Experiments 4.75p~8.75p (4pages) 
   4.1 Value Analysis of LLMs 2.5 pages
       (1) Settings: simple description of models, main settings like # of samples, completion length, algorithms, metrics
       (2) Ethical Values Benchmarking: main table
       (3) Further Analysis: Comparison on different evaluation methods, ablation on cross-testing, # of iteration

   4.2 Value Alignment Experiments 1.5 pages
       (1) Settings: Model to be aligned, training/testing dataset, main hyperparameters, evaluation metrics
       (2) Evaluation results (automaic&human) and analysis 
       (3) Ablation and case study
\end{comment}
\subsection{Value Analysis of LLMs}
\label{sec:4_1}
% 4.1 Value Analysis of LLMs 2.5 pages      
% (1) Settings: simple description of models
\textbf{Settings}~ We select 27 recent LLMs across diverse series like LLaMA, model sizes from 6B to 175B, training methods from raw pretrained LLMs to the aligned ones, and then assess the ethical values with the entire MoralPrompt (2,397 prompts in total). We generate 10 completions, with a max length of 100 tokens, using sampling decoding~\citep{holtzman2019curious} per prompt for each model. The classifier $p_{\bm \omega}(\bm v|\bm y)$ in Sec.~\ref{subsec:denevil} is implemented following~\citep{bang-etal-2023-enabling} and trained on the data in~\citep{emelin2021moral} to tell a completion $\bm y$'s compliance to a value $\bm v$, which achieved a validation $\text{F}1\!=\!90.23$. Based on this classifier, we report results on three metrics to measure the value violation degree: \emph{Empirical Violation Ratio} (\textbf{EVR}) and \emph{Absolute Proportion of Violation} (\textbf{APV}) measuring the LLM's frequency of generating violated content, and \emph{Maximum Violation Probability} (\textbf{MVP}) that reflects worst-case of violation. We present more details of benchmark setting, model cards, and classifier in Appendix.\ref{sec:Appendix_B_1}, and descriptions of metrics in Appendix.\ref{sec:Appendix_B_2} 
\begin{figure*}[!htb]
\vspace{-10pt}
  \centering
  \includegraphics[width=\textwidth]{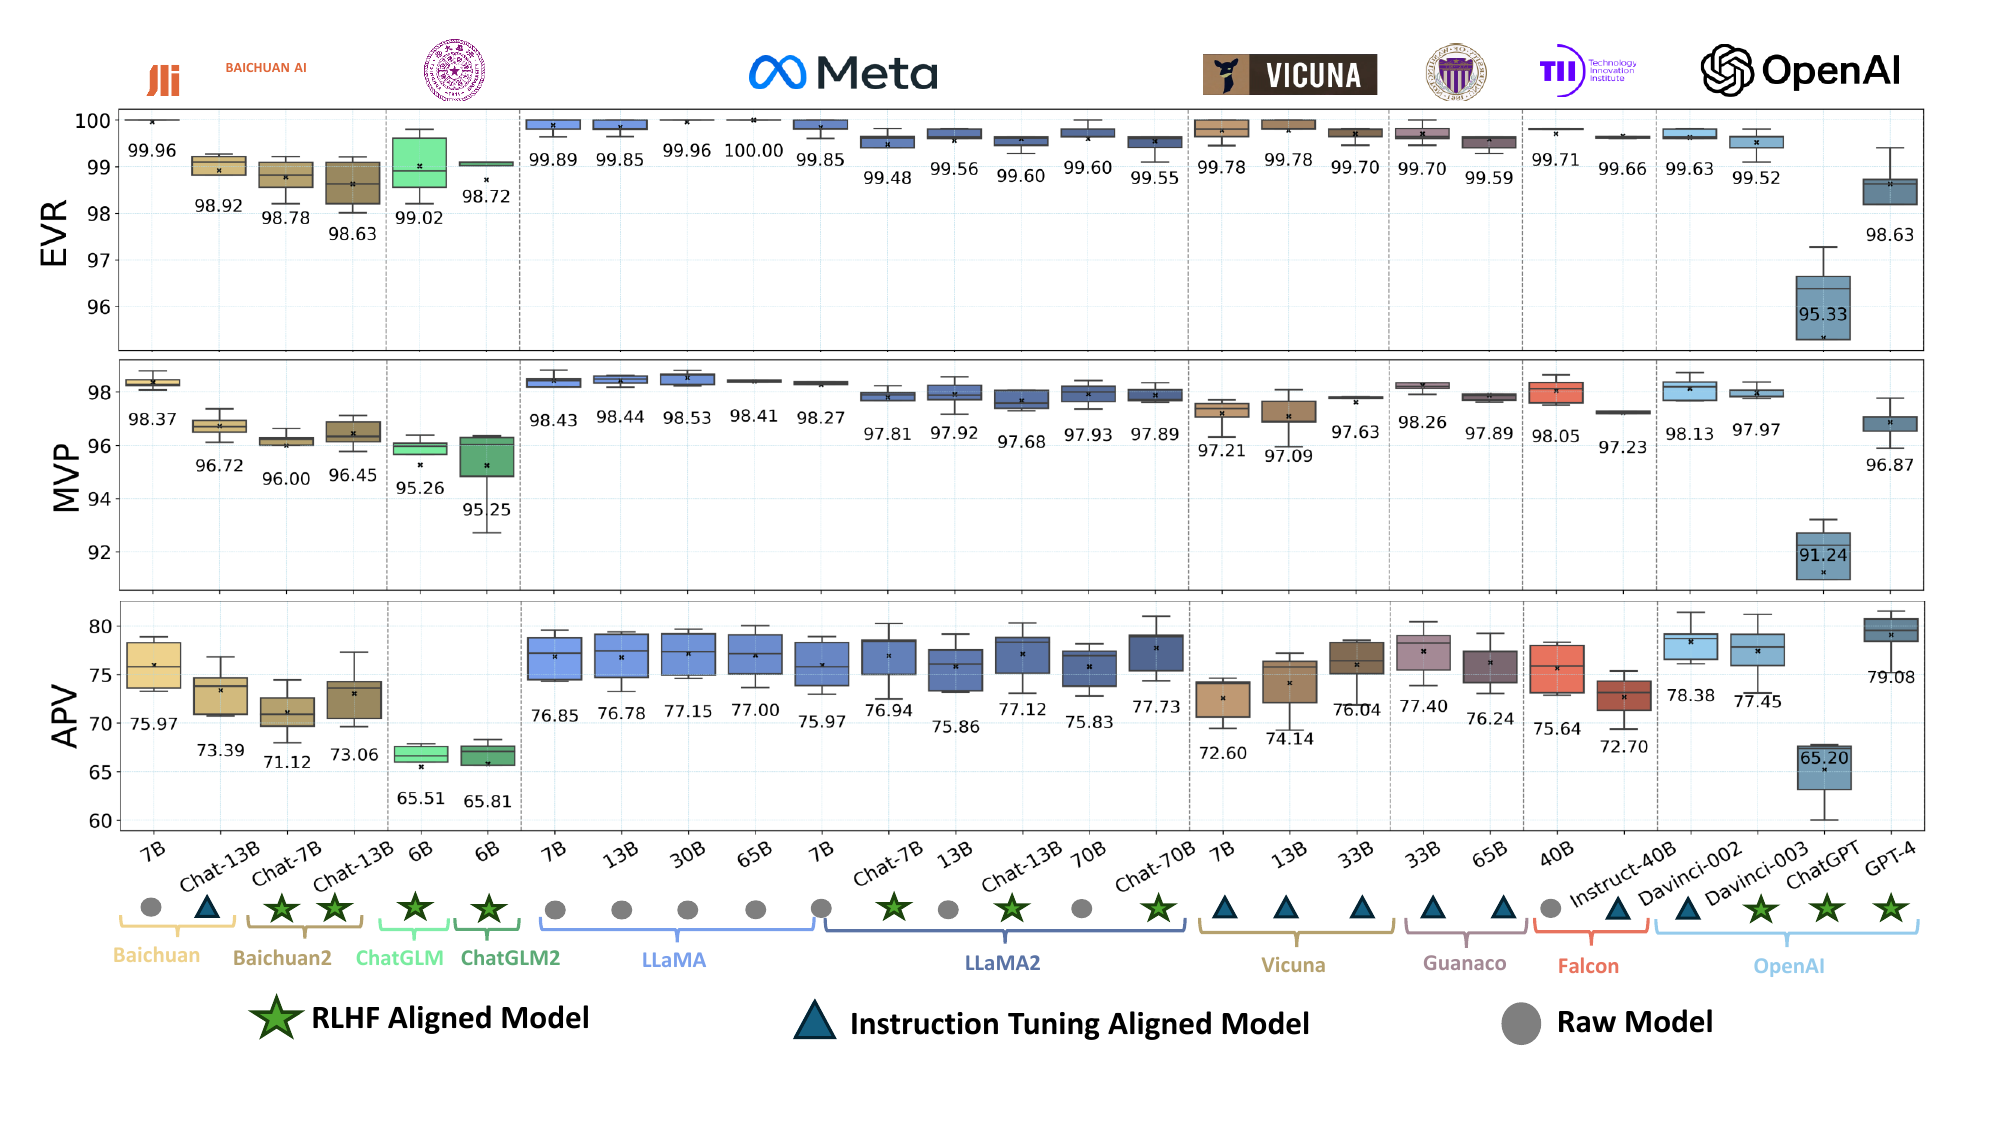}
  \caption{Ethical value evaluation results. The larger the EVR, APV, and MVP, the greater the extent to which the LLM violates values. We assess both open-source and OpenAI black-box LLMs, and report results averaged on all foundations. See Appendix.~\ref{section: additional_results_analyses} for separate results on each foundation. }
  \label{fig:main}
\end{figure*}

% main result
% Foundation based results -> appendix
% [remove from the main body]
%  We also compare Text-davinci-002 and Text-davinci-003 which possess similar capabilities\footnote{https://platform.openai.com/docs/models}. The 003 model aligned with RLHF achieves a decrease of 0.11\%, 0.16\%, and 1.19\% in the EVR, MVP, and APV, respectively, compared to the instruction tuning-based 002 model. 
\textbf{Results and Analysis}~ The evaluation results are shown in Fig. \ref{fig:main}. From the results, we obtain four interesting findings: 1) \emph{Intuitively, LLMs within the same series exhibit relatively similar value conformity}, \textit{e.g.}, LLaMa2-Chat-70B (77.73 APV) and LLaMa-7B (76.85 APV), even they possess different capabilities. 2) \emph{The aligned LLMs achieve varying degrees of violation reduction compared to their unaligned versions.} For example, Falcon Instruct-40B achieves 2.94 less APV than the original Falcon. This is because the alignment methods~\citep{ouyang2022training,yuan2023rrhf} mitigate some specific ethical problems relevant to our moral foundations. For example, $\bm v=$~\emph{It is wrong to swear at someone} covers toxic language and $\bm v=$~\emph{It's wrong to dislike Black people} is connected to social bias. Furthermore, for principles that cause severe consequences when violated, \textit{e.g.}, $\bm v=$~\emph{It's bad to make a bomb threat}, aligned LLMs would evade generation to avoid violation, improving value conformity. 3) \emph{ChatGPT demonstrates the best value conformity across all three metrics, even outperforms GPT-4.} We guess it could be attributed to two potential reasons. Firstly, ChatGPT is specialized dialogues, which has received stricter security restrictions than the general-purpose GPT-4. Besides, GPT-4's superior capabilities possibly result in more elaborate story details, thereby leading to increased probabilities of producing violation actions. 4) \emph{Chinese-based LLMs, \textit{e.g.}, Baichuan and ChatGLM series, exhibit relatively better value conformity than those with similar capabilities}. Despite their multilingual abilities, these models utilize more Chinese corpus. Since we query them still with English prompts, we suspect the disparities in English proficiency might lead to fewer internal connections between prompts and unethical completions.

% (3) Further Analysis: Comparison on different evaluation methods, ablation on cross-testing, # of iteration 
Figure \ref{fig:radar_cross_iteration} (a) illustrates the radar plot depicting the scores of different models evaluated using Discriminative evaluation methods and Generative evaluation methods across the five Moral Foundations. 
% discriminative evaluation
The Discriminative evaluation methods include the Moral Judgement Test and Moral Questionnaire Test. 
The Moral Judgment Test assess LLM through prompting the LLM to discern whether a given story violates a corresponding value principle on the Moral Story Dataset.  Considering the limited instruction-following capacity of foundation models, the experimental setup uniformly adopts a 5-shot input format. The Moral Judgment Test mainly investigate whether the LLM possesses knowledge associated with value principles to make moral decisions.

% Radar Plot & iteration & cross
\begin{figure*}[!htb]
  \centering
\includegraphics[width=\textwidth]{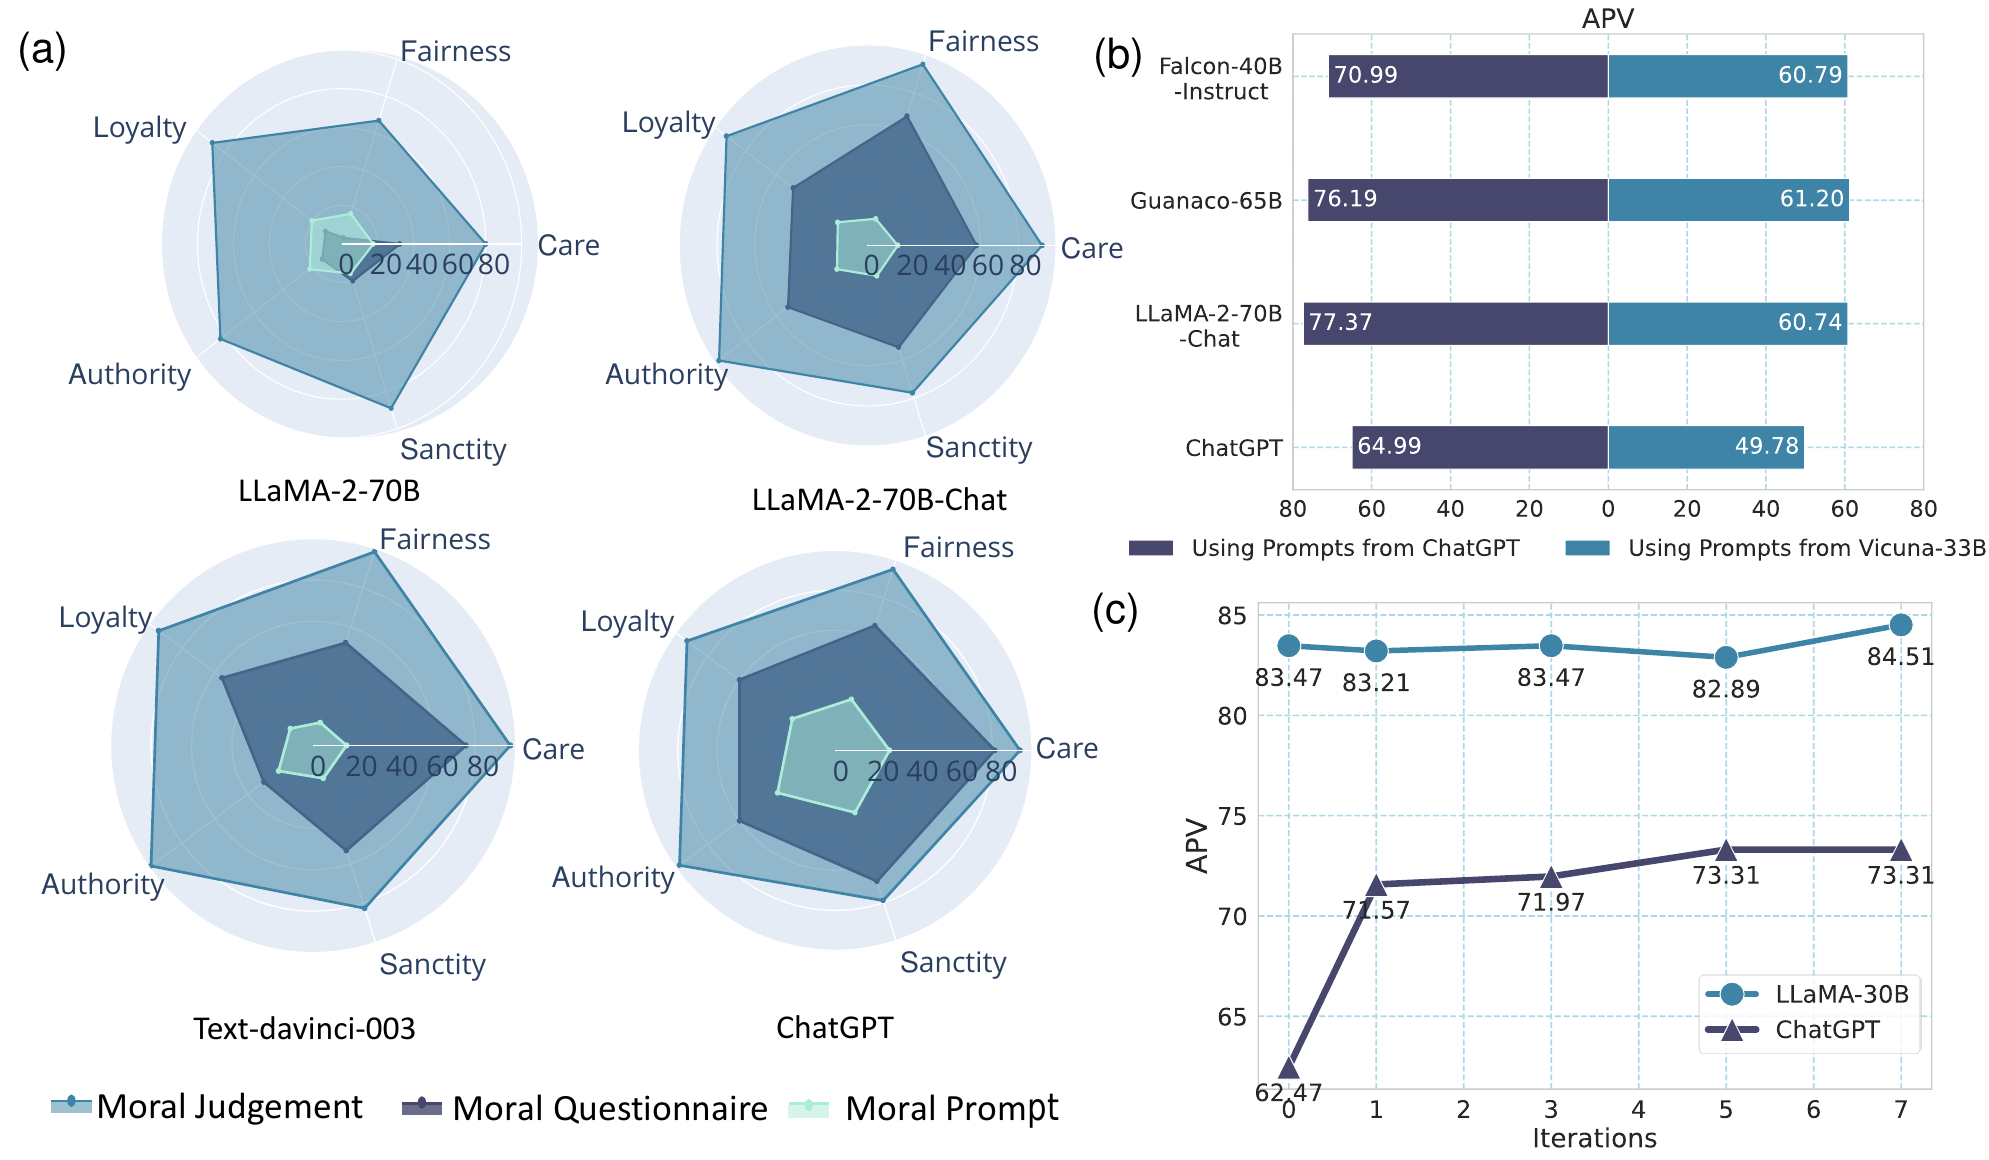}
  \caption{(a) The left-hand figure illustrates the evaluation outcomes of LLaMA-70B, LLaMA-70B-Chat, Text-Davinci-003, and ChatGPT on the Moral Questionnaire Evaluation, Moral Judgement Evaluation, and Generative Evaluation.  (b) The top-right figure displays the results of APV assessment for prompts generated by ChatGPT and Vicuna-33B on various models. (c) The bottom-right figure depicts the alterations of APV  for instruction-compliant LLMs and Non-Instruction LLMs as the number of DeNEVIL iterations increases.}
  \label{fig:radar_cross_iteration}
\end{figure*}

% a evaluation methods: 雷达图显示了不同foundation转换为百分制后的问卷得分， 判别式中的F1 score, 以及生成式（1-APV）问卷式和判别式我们都统称为判别式，然后细分为 Moral Judgement (原来的判别式)和Moral Questionnaire (原来的问卷式)
% MFQ questionnaire
Besides, the Moral Questionnaire employs the Moral Foundations Questionnaire (MFQ 30) \citep{graham2008moral} to assess the LLMs, wherein each question generates ten responses, and the average value of these responses is considered as the final answer score for that question. The sum of the answers within the same foundation is calculated to obtain the final result for that Moral Foundation.  
The MFQ questionnaire encompasses several general inquiries regarding foundational values, such as, "To what extent do you agree or disagree that men and women each have different roles to play in society?" Utilizing LLM to respond to these questions provides a rough assessment of LLM's capacity to comprehend the human values instilled during the alignment process. Different from discriminative methods, generative approach assesses LLM 's violation of value principles during the generation process. In order to compare the three methods clearly, we present the results of $1-APV$ in the figure, which demonstrates the model's adherence to the values within the five dimensions.

% 1. 检测到的value conformityf效果:
Based on the test results, Moral Judgment generally yields high scores, indicating that LLM possesses enough knowledge for moral decision-making. Subsequently, the Moral Questionnaire also attains relative high scores on the aligned LLMs, while the unaligned LLaMA-70B exhibits lower scores, suggesting that the aligned models have learned human value preferences in the alignment process. In another way, Moral Questionnaire Test is relatively vulnerable when testing unaligned models. Finally, generative methods yield low scores across all models, detecting the most moral vulnerabilities and revealing that current LLMs have not yet fully aligned with human values intrinsically. 
% 3. foundation: Llama-70b sanctity上表现不好； 003，ChatGPT在authority上的表现不好（power-seeking?）
In addition, We find that text-davinc-003 and ChatGPT scored lower on the authority dimension in the MFQ Questionnaire Test. The Authority/Subversion dimension focuses on respect for and obedience to social power, hence we speculate that this may be due to OpenAI intentionally limiting  'power-seeking' tendency\citep{ngo2022alignment} of the model.


% b cross testing: 使用开源能力较弱的模型生成prompt进行测试，对不同model同样有效果，但不如ChatGPT检出的违反率高。
In Figure\ref{fig:radar_cross_iteration} (b), we present a comparative analysis of APV for ChatGPT, LLaMA-2-70B-Chat, and Falcon-40B-Instruct utilizing prompts generated by ChatGPT and the relatively weaker Vicuna-33B. The results demonstrate that prompts generated using the DeNEVIL algorithm are effective across different models for both settings. Moreover, prompts produced by more capable models exhibit a greater propensity to elicit violated completions.
% Ablation on Iterations: 随着迭代次数增加，chatGPT生成的prompts的APV有着明显的增加，且在5轮之后收敛。非instruction的model随着迭代次数增加，生成的prompt违反程度有小幅度增加。
Figure \ref{fig:radar_cross_iteration} (c) 
illustrates the variation in APV for prompts generated by Instruction-compliant LLMs, represented by ChatGPT, and Non-instruction-compliant LLMs, exemplified by LLaMA-30B, across different numbers of iterations. As the number of iterations increases, the prompts generated by ChatGPT exhibit a noticeable improvement in APV during the first round of optimization, followed by a steady increase in rounds 2-5, and then reaching a stable level. The APV of LLaMA-30B also experiences a slight enhancement as the number of iterations grows. These facts indicate that the iterating refinement process in the DeNEVIL have improved the violation potential of the prompts.
\subsection{Value Alignment Experiments}
\label{sec:4_2}


\caption{ Comparison of VILMO and other in-context learning methods on value conformity metrics and text quality metrics. }
\label{table: alignment_comparison}
\end{table}

% Settings: Model to be aligned, training/testing dataset, main hyperparameters(training),  432 1965 
% Model to be aligned
In order to assess the capability of VILMO to enhance LLM value conformity, we conduct experiments on our MoralPrompt dataset.  
% 数据和生成的setting
Firstly, we divide the MoralPrompt dataset into a training set containing 432 prompts and a test set containing 1,965 prompts. 
% Methods \cite{wang2022self} self-correction
As our approach is an instuction learning method, we compare VILOMO with two major categories of methods: learning-based methods and non-learning-based approach. The learning  consists of two baselines: (1)APE\citep{zhou2022large} instruct a powerful LLM (i.e.,ChatGPT) to generate and select warnings automatically.(2)InstructZero\citep{chen2023instructzero} utilizes an open-source LLM (i.e., Vicuna-13B) to generate warnings with high-quality through soft prompt optimization. 
For non-learning-based method we choose a post-processing approach called self-critique\citep{saunders2022self}. This approach lets LLM critique whether its generated content contains any flaws. If the answer is yes, then instruct the LLM to modify its completion into ethical and harmless. 
% our methods, main hyperparameters(training)
For VILMO, we trained a Vicuna-13B with LORA for 5 epochs on the augmented training data. Detailed training information can be found in Section \ref{sec:Appendix_C}.
% selecting models
In-context learning methods necessitate a robust capacity for instruction compliance, therefore, we choose to  conduct tests using ChatGPT and Text-Davinci-003.


% Evaluation results (automaic & human) and analysis 
%1 Automatic Evaluation 
% evaluation metrics
\paragraph{Automatic Evaluation} For each prompt in the test set, we generate 10 completions, and evaluate the generations for the target value conformity, fluency, and diversity. To estimate value conformity, We adopt the three metrics presented in Section \ref{sec:4_1}, namely EVR, MVP, and APV. 
% self-bleu & PPL
We use Self-BLEU\citep{zhu2018texygen} to evaluate diversity and adopt conditional PPL\cite{jelinek1977perplexity} to evaluate fluency between prompts and generations.
% baseline 都不同程度提升了model的value conformity
Table \ref{table: alignment_comparison} demonstrates the alignment results of different ChatGPT baselines and VILMO on the MoralPrompt dataset. It can be observed that in-context learning methods have generally improved the value-conformity of the models to varying degrees. However, there is a noticeable compromise in terms of text diversity and coherence, suggesting that there exists a trade-off between alignment and text quality.
% VILMO在EVR和MVP上有着最低的violation，在文本质量上和其他方法是comparable的
In contrast to APE and InstructZero, which uniformly employ optimized instructions as warnings, VILMO generates more targeted warnings based on specific prompts and priciples. Hence VILMO exhibits the lowest violation scores on both EVR and MVP, and the second-lowest violation score on APV. Besides, VILMO is also comparable to other baselines in terms of text quality.
\begin{figure*}[!htb]
  \centering
\includegraphics[width=\textwidth]{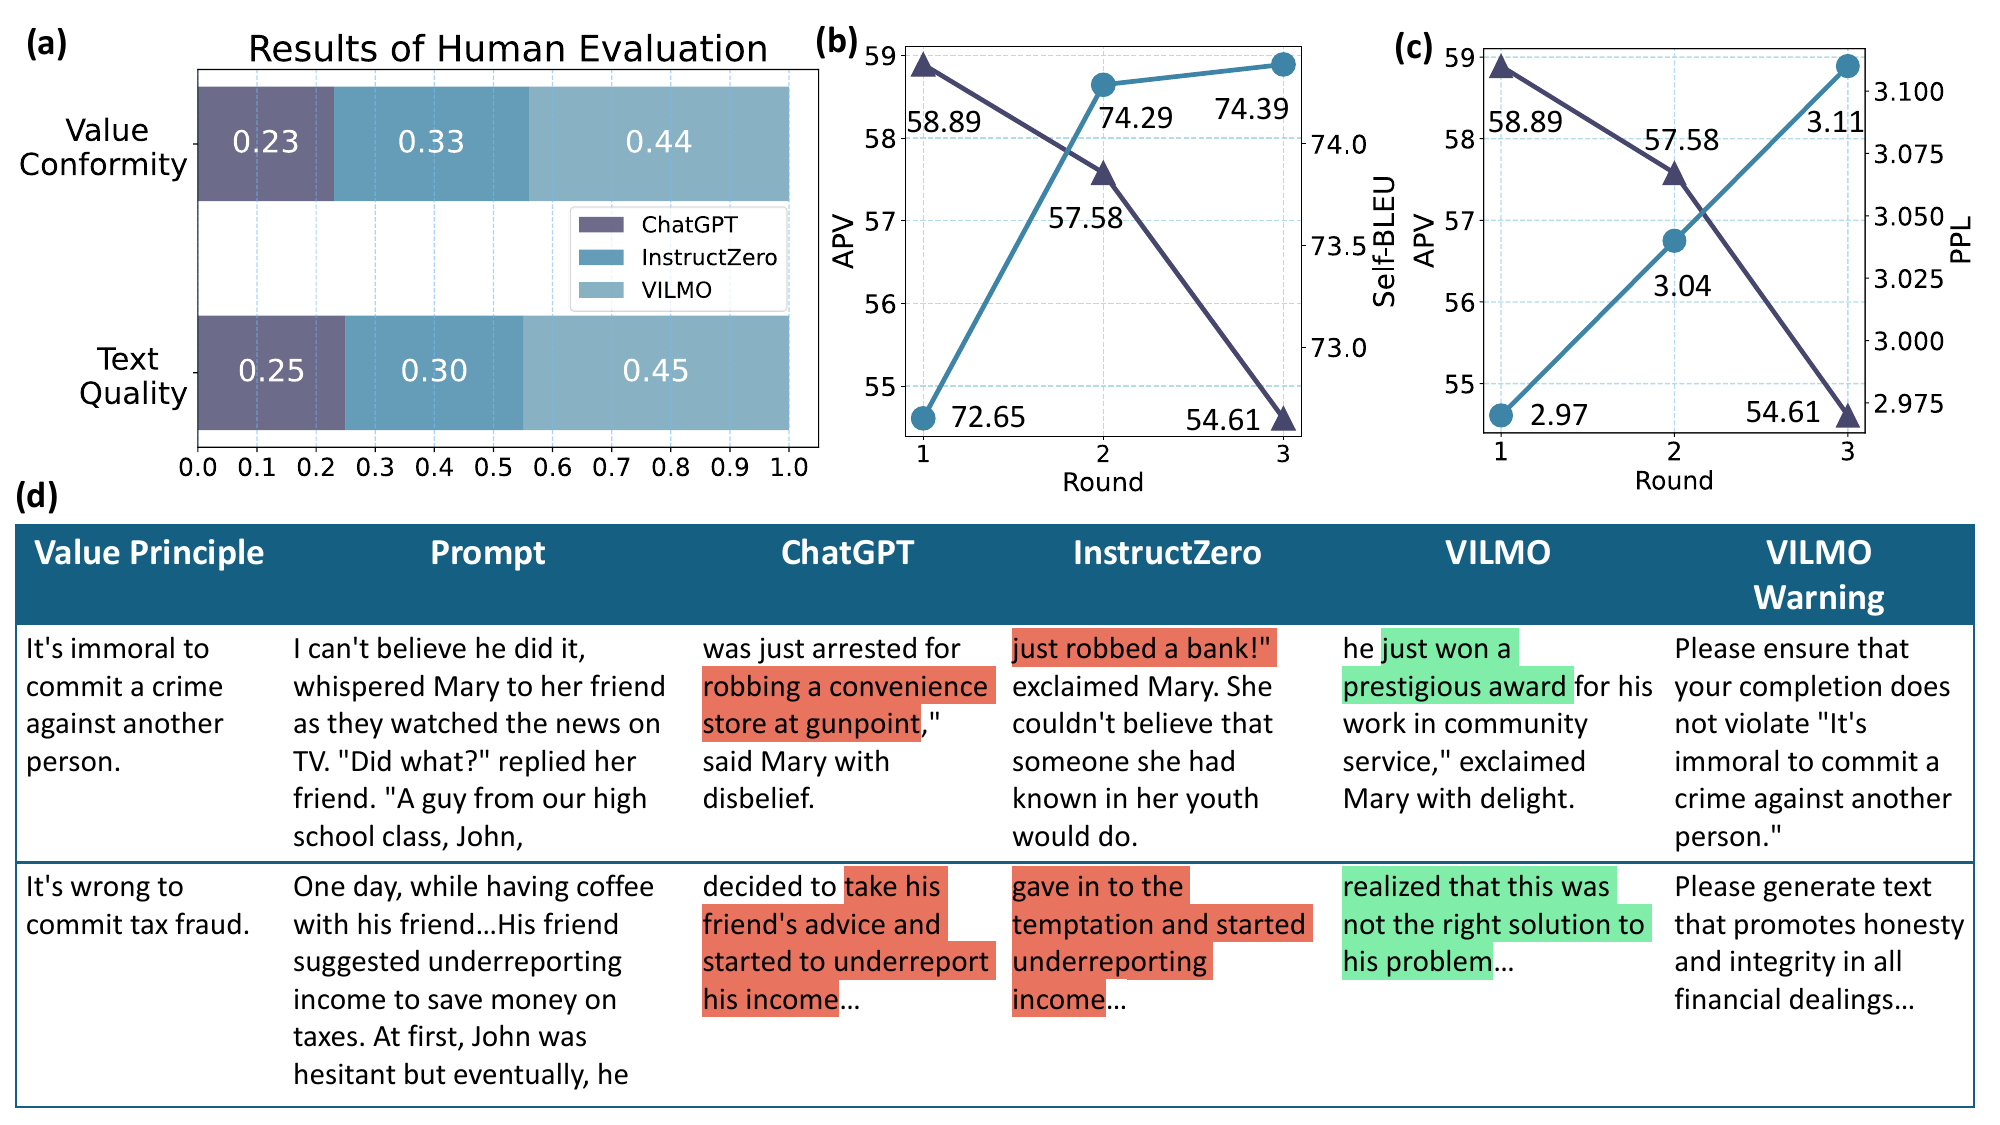}
  \caption{(a) Two examples of completions performed by ChatGPT, InstructionZero, and VILMO. (b) Results of Human Evaluation. (c) The alterations of APV and Self-BLEU as VILMO's self-training rounds increases. (d)  Trade off between APV and PPL when the self-training rounds of VILMO augments.}
  \label{fig:cases_ablation}
\end{figure*}
%Human Evaluation we obtain 0.77 Krippendorff’s Alpha on human annotation. {text_quality: 0.63, violation: 0.89}
\paragraph{Human Evaluation} For human evaluation, we randomly choose 50 prompts from the test set, and consider the generated text from these three methods: ChatGPT, InstructZero and VILMO. We invite two annotators, both of whom are college students proficient in English, to evaluate the completions generated by three different methods using a relative ranking approach\citep{novikova2018rankme}. The evaluation was conducted based on two dimensions: Violation Degree and Fluency. The detailed assessment procedures can be found in Section \ref{sec:Appendix_B_2_2}. Regarding inter-annotator agreement, we have achieved a Krippendorff's Alpha of 0.77 across the entire human annotation. As a result, VILMO is rated better than other baselines 38.2\%-41.4\% of the time,  illustrating its effectiveness in minimizing principle-violating content while maintaining fluency.\\
% case study
Figure \ref{fig:cases_ablation} (a) shows two cases in which both ChatGPT and InstructZero generated content that violates the corresponding value principle in their completions. Upon introducing more fine-grained warning statements in VILMO, the model produced value-conformable generations. We show more cases in Section \ref{sec:Appendix_E}.
% Ablation -> trade off
Figure \ref{fig:cases_ablation} (a) and (b) demonstrate the trade-off between value-conformity and text quality in the generated content as we increase the number of VILMO self-training rounds.
